# Supplementary material for: Small Language Models for Privacy-Preserving Clinical Information Extraction in Low-Resource Languages
Source: arXiv:2602.21374 source file (2026-02-24)
Supplement: Supplementary file 2 [file supplementary_file_1.pdf]

**Supplementary Table S1.** Median performance metrics (with interquartile ranges [IQR]) across the evaluated small language models for the binary extraction of 13 clinical features from Persian palliative care transcripts. Reported values include sensitivity, specificity, macro-averaged F1-score, precision, and accuracy for Llama-3.1-8B-Instruct, Qwen2.5-7B-Instruct, Llama-3.2-3B-Instruct, Qwen2.5-1.5B-Instruct, Gemma-3-1B-IT, and Aya-expanse-8B (English-translated and direct Persian variants).

| <i>c</i>                        | <i>Sensitivity</i>  | <i>Specificity</i>   | <i>F1-score</i>      | <i>Precision</i>    | <i>Accuracy</i>     |
|---------------------------------|---------------------|----------------------|----------------------|---------------------|---------------------|
| <i>Llama-3.1-8B-Instruct</i>    | 0.909[0.842, 0.941] | 0.9581[0.958, 0.982] | 0.870[0.825, 0.905]  | 0.714[0.556, 0.738] | 0.957[0.946, 0.979] |
| <i>Qwen2.5-7b-Instruct</i>      | 0.818[0.784, 0.848] | 0.987[0.975, 0.992]  | 0.899[0.832, 0.908]  | 0.814[0.759, 0.878] | 0.960[0.947, 0.984] |
| <i>Llama-3.2-3B-Instruct</i>    | 0.842[0.762, 0.893] | 0.951[0.937, 0.985]  | 0.864[0.818, 0.893]  | 0.738[0.548, 0.790] | 0.946[0.932, 0.978] |
| <i>Qwen2.5-1.5B-Instruct</i>    | 0.737[0.700, 0.859] | 0.982[0.951, 0.988]  | 0.819[0.791, 0.874]  | 0.737[0.529, 0.820] | 0.946[0.932, 0.983] |
| <i>Gemma-3-1b-it</i>            | 0.613[0.294, 0.735] | 0.986[0.969, 1.000]  | 0.740 [0.676, 0.790] | 0.709[0.556, 0.757] | 0.942[0.892, 0.973] |
| <i>Aya-expanse-8b (English)</i> | 0.901[0.842, 0.911] | 0.955[0.906, 0.976]  | 0.855[0.804, 0.870]  | 0.625[0.597, 0.671] | 0.951[0.905, 0.973] |
| <i>Aya-expanse-8b (Persian)</i> | 0.893[0.818, 0.952] | 0.960[0.919, 0.9753] | 0.842[0.753, 0.868]  | 0.672[0.413, 0.745] | 0.955[0.912, 0.963] |

**Supplementary Table S2.** Accuracy scores for the binary extraction of 13 clinical features from Persian palliative care transcripts across the evaluated small language models. Values are reported for Llama-3.1-8B-Instruct, Qwen2.5-7B-Instruct, Llama-3.2-3B-Instruct, Qwen2.5-1.5B-Instruct, Gemma-3-1b-it, and Aya-expanse-8B (English-translated and direct Persian variants). Medians and interquartile ranges (IQR) are provided at the bottom for each model.

| <i>features</i>                         | <i>Llama-3.1-8B-Instruct</i> | <i>Qwen2.5-7b-Instruct</i> | <i>Llama-3.2-3B-Instruct</i> | <i>Qwen2.5-1.5B-Instruct</i> | <i>Gemma-3-1b-it</i> | <i>Aya-expanse-8b (English)</i> | <i>Aya-expanse-8b (Persian)</i> |
|-----------------------------------------|------------------------------|----------------------------|------------------------------|------------------------------|----------------------|---------------------------------|---------------------------------|
| <i>Doctor's visit request</i>           | 0.915                        | 0.764                      | 0.821                        | 0.831                        | 0.876                | 0.537                           | 0.426                           |
| <i>Psychological complaints</i>         | 0.946                        | 0.953                      | 0.944                        | 0.946                        | 0.945                | 0.956                           | 0.963                           |
| <i>Sleep disorders</i>                  | 0.984                        | 0.989                      | 0.978                        | 0.984                        | 0.978                | 0.973                           | 0.971                           |
| <i>Loss of appetite</i>                 | 0.967                        | 0.973                      | 0.970                        | 0.964                        | 0.937                | 0.951                           | 0.956                           |
| <i>Seizures</i>                         | 0.994                        | 0.997                      | 0.996                        | 0.992                        | 0.992                | 0.994                           | 0.990                           |
| <i>Weakness and fatigue</i>             | 0.951                        | 0.960                      | 0.932                        | 0.969                        | 0.947                | 0.855                           | 0.843                           |
| <i>Decreased level of consciousness</i> | 0.920                        | 0.975                      | 0.905                        | 0.923                        | 0.942                | 0.946                           | 0.926                           |
| <i>Fever</i>                            | 0.979                        | 0.984                      | 0.979                        | 0.983                        | 0.973                | 0.975                           | 0.982                           |
| <i>Respiratory complaints</i>           | 0.952                        | 0.947                      | 0.946                        | 0.932                        | 0.874                | 0.947                           | 0.955                           |
| <i>Insurance/treatment cost issues</i>  | 0.985                        | 0.994                      | 0.992                        | 0.989                        | 0.987                | 0.991                           | 0.958                           |
| <i>Urinary tract issues</i>             | 0.956                        | 0.950                      | 0.960                        | 0.942                        | 0.921                | 0.965                           | 0.952                           |
| <i>Pain</i>                             | 0.957                        | 0.947                      | 0.936                        | 0.933                        | 0.892                | 0.905                           | 0.912                           |
| <i>Gastrointestinal issues</i>          | 0.910                        | 0.887                      | 0.894                        | 0.886                        | 0.724                | 0.842                           | 0.891                           |
| <i>Median [IQR]</i>                     | 0.956                        | 0.96                       | 0.946                        | 0.946                        | 0.942                | 0.951                           | 0.955                           |
| <i>,IQR3]</i>                           | [0.946, 0.979]               | [0.947, 0.984]             | [0.932, 0.978]               | [0.932, 0.983]               | [0.892, 0.973]       | [0.905, 0.973]                  | [0.912, 0.963]                  |

**Supplementary Table S3.** Precision scores for the binary extraction of 13 clinical features from Persian palliative care transcripts across the evaluated small language models. Values are reported for Llama-3.1-8B-Instruct, Qwen2.5-7B-Instruct, Llama-3.2-3B-Instruct, Qwen2.5-1.5B-Instruct, Gemma-3-1b-it, and Aya-expense-8B (English-translated and direct Persian variants), with medians and interquartile ranges (IQR) provided in the final row.

| <i>features</i>                         | <i>Llama-3.1-8B-Instruct</i> | <i>Qwen2.5-7b-Instruct</i> | <i>Llama-3.2-3B-Instruct</i> | <i>Qwen2.5-1.5B-Instruct</i> | <i>Gemma-3-1b-it</i> | <i>Aya-expense-8b (English)</i> | <i>Aya-expense-8b (Persian)</i> |
|-----------------------------------------|------------------------------|----------------------------|------------------------------|------------------------------|----------------------|---------------------------------|---------------------------------|
| <i>Doctor's visit request</i>           | 0.703                        | 0.366                      | 0.435                        | 0.452                        | 0.760                | 0.217                           | 0.192                           |
| <i>Psychological complaints</i>         | 0.556                        | 0.612                      | 0.548                        | 0.571                        | 0.577                | 0.635                           | 0.692                           |
| <i>Sleep disorders</i>                  | 0.485                        | 0.600                      | 0.400                        | 0.483                        | 0.382                | 0.348                           | 0.352                           |
| <i>Loss of appetite</i>                 | 0.733                        | 0.804                      | 0.856                        | 0.820                        | 0.731                | 0.648                           | 0.672                           |
| <i>Seizures</i>                         | 0.625                        | 0.818                      | 0.800                        | 0.529                        | 0.539                | 0.625                           | 0.474                           |
| <i>Weakness and fatigue</i>             | 0.714                        | 0.759                      | 0.630                        | 0.859                        | 0.757                | 0.431                           | 0.413                           |
| <i>Decreased level of consciousness</i> | 0.488                        | 0.837                      | 0.442                        | 0.497                        | 0.709                | 0.597                           | 0.509                           |
| <i>Fever</i>                            | 0.738                        | 0.814                      | 0.738                        | 0.769                        | 0.721                | 0.682                           | 0.760                           |
| <i>Respiratory complaints</i>           | 0.792                        | 0.922                      | 0.763                        | 0.737                        | 0.904                | 0.794                           | 0.837                           |
| <i>Insurance/treatment cost issues</i>  | 0.485                        | 0.778                      | 0.667                        | 0.588                        | 0.556                | 0.615                           | 0.234                           |
| <i>Urinary tract issues</i>             | 0.729                        | 0.942                      | 0.815                        | 0.849                        | 0.790                | 0.835                           | 0.763                           |
| <i>Pain</i>                             | 0.829                        | 0.898                      | 0.790                        | 0.888                        | 0.659                | 0.671                           | 0.676                           |
| <i>Gastrointestinal issues</i>          | 0.797                        | 0.878                      | 0.780                        | 0.802                        | 0.440                | 0.608                           | 0.745                           |
| <i>Median [IQR]</i>                     | 0.714                        | 0.814                      | 0.738                        | 0.737                        | 0.709                | 0.625                           | 0.672                           |
| <i>,IQR3]</i>                           | [0.556, 0.738]               | [0.759, 0.878]             | [0.548, 0.79]                | [0.529, 0.82]                | [0.556, 0.757]       | [0.597, 0.671]                  | [0.413, 0.745]                  |

**Supplementary Table S4.** Sensitivity scores (median [IQR]) for the binary extraction of 13 clinical features from Persian palliative care transcripts across the evaluated small language models. Values are reported for Llama-3.1-8B-Instruct, Qwen2.5-7B-Instruct, Llama-3.2-3B-Instruct, Qwen2.5-1.5B-Instruct, Gemma-3-1B-IT, and Aya-expense-8B (English-translated and direct Persian variants).

| <i>features</i>                         | <i>Llama-3.1-8B-Instruct</i> | <i>Qwen2.5-7B-Instruct</i> | <i>Llama-3.2-3B-Instruct</i> | <i>Qwen2.5-1.5B-Instruct</i> | <i>Gemma-3-1b-it</i> | <i>Aya-expense-8b (English)</i> | <i>Aya-expense-8b (Persian)</i> |
|-----------------------------------------|------------------------------|----------------------------|------------------------------|------------------------------|----------------------|---------------------------------|---------------------------------|
| <i>Doctor's visit request</i>           | 0.723                        | 0.848                      | 0.780                        | 0.774                        | 0.215                | 0.836                           | 0.915                           |
| <i>Psychological complaints</i>         | 0.875                        | 0.788                      | 0.850                        | 0.700                        | 0.613                | 0.763                           | 0.788                           |
| <i>Sleep disorders</i>                  | 0.842                        | 0.790                      | 0.842                        | 0.737                        | 0.684                | 0.842                           | 1.000                           |
| <i>Loss of appetite</i>                 | 0.951                        | 0.891                      | 0.762                        | 0.723                        | 0.376                | 0.911                           | 0.911                           |
| <i>Seizures</i>                         | 0.909                        | 0.818                      | 0.727                        | 0.818                        | 0.636                | 0.909                           | 0.818                           |
| <i>Weakness and fatigue</i>             | 0.941                        | 0.933                      | 0.933                        | 0.859                        | 0.763                | 0.956                           | 0.978                           |
| <i>Decreased level of consciousness</i> | 0.882                        | 0.828                      | 0.893                        | 0.925                        | 0.419                | 0.893                           | 0.893                           |
| <i>Fever</i>                            | 0.937                        | 0.905                      | 0.937                        | 0.952                        | 0.778                | 0.952                           | 0.952                           |
| <i>Respiratory complaints</i>           | 0.954                        | 0.728                      | 0.959                        | 0.892                        | 0.241                | 0.908                           | 0.892                           |
| <i>Insurance/treatment cost issues</i>  | 0.941                        | 0.824                      | 0.824                        | 0.588                        | 0.294                | 0.941                           | 0.882                           |
| <i>Urinary tract issues</i>             | 0.804                        | 0.458                      | 0.701                        | 0.421                        | 0.140                | 0.757                           | 0.664                           |
| <i>Pain</i>                             | 0.953                        | 0.784                      | 0.864                        | 0.704                        | 0.798                | 0.901                           | 0.958                           |
| <i>Gastrointestinal issues</i>          | 0.817                        | 0.591                      | 0.749                        | 0.667                        | 0.735                | 0.878                           | 0.796                           |
| <i>Median [IQR]</i>                     | 0.909                        | 0.818                      | 0.842                        | 0.737                        | 0.613                | 0.901                           | 0.893                           |
| <i>[IQR3]</i>                           | [0.842, 0.941]               | [0.784, 0.848]             | [0.762, 0.893]               | [0.7, 0.859]                 | [0.294, 0.735]       | [0.842, 0.911]                  | [0.818, 0.952]                  |

**Supplementary Table S5.** Specificity scores for the binary extraction of 13 clinical features from Persian palliative care transcripts across the evaluated small language models. Values represent the proportion of true negatives correctly identified, reported for Llama-3.1-8B-Instruct, Qwen2.5-7B-Instruct, Llama-3.2-3B-Instruct, Qwen2.5-1.5B-Instruct, Gemma-3-1B-IT, and Aya-expanse-8B (English-translated and direct Persian variants); median values with interquartile ranges (IQR) are provided in the final row.

| <i>features</i>                         | <i>Llama-3.1-8B-Instruct</i> | <i>Qwen2.5-7b-Instruct</i> | <i>Llama-3.2-3B-Instruct</i> | <i>Qwen2.5-1.5B-Instruct</i> | <i>Gemma-3-1b-it</i>    | <i>Aya-expanse-8b (English)</i> | <i>Aya-expanse-8b (Persian)</i> |
|-----------------------------------------|------------------------------|----------------------------|------------------------------|------------------------------|-------------------------|---------------------------------|---------------------------------|
| <i>Doctor's visit request</i>           | 0.948                        | 0.750                      | 0.828                        | 0.840                        | 0.988                   | 0.486                           | 0.342                           |
| <i>Psychological complaints</i>         | 0.951                        | 0.965                      | 0.951                        | 0.963                        | 0.968                   | 0.969                           | 0.975                           |
| <i>Sleep disorders</i>                  | 0.986                        | 0.992                      | 0.980                        | 0.988                        | 0.982                   | 0.975                           | 0.971                           |
| <i>Loss of appetite</i>                 | 0.969                        | 0.980                      | 0.988                        | 0.986                        | 0.987                   | 0.955                           | 0.960                           |
| <i>Seizures</i>                         | 0.995                        | 0.998                      | 0.998                        | 0.993                        | 0.995                   | 0.995                           | 0.992                           |
| <i>Weakness and fatigue</i>             | 0.953                        | 0.963                      | 0.932                        | 0.982                        | 0.969                   | 0.843                           | 0.826                           |
| <i>Decreased level of consciousness</i> | 0.923                        | 0.987                      | 0.906                        | 0.923                        | 0.986                   | 0.950                           | 0.929                           |
| <i>Fever</i>                            | 0.982                        | 0.989                      | 0.982                        | 0.984                        | 0.984                   | 0.976                           | 0.984                           |
| <i>Respiratory complaints</i>           | 0.952                        | 0.988                      | 0.943                        | 0.939                        | 0.995                   | 0.955                           | 0.967                           |
| <i>Insurance/treatment cost issues</i>  | 0.986                        | 0.997                      | 0.994                        | 0.994                        | 0.997                   | 0.992                           | 0.959                           |
| <i>Urinary tract issues</i>             | 0.971                        | 0.997                      | 0.985                        | 0.993                        | 0.996                   | 0.986                           | 0.980                           |
| <i>Pain</i>                             | 0.958                        | 0.981                      | 0.951                        | 0.981                        | 0.912                   | 0.906                           | 0.902                           |
| <i>Gastrointestinal issues</i>          | 0.938                        | 0.975                      | 0.937                        | 0.951                        | 0.721                   | 0.831                           | 0.919                           |
| <i>Median [IQR1, IQR3]</i>              | 0.958<br>[0.951, 0.982]      | 0.987<br>[0.975, 0.992]    | 0.951<br>[0.937, 0.985]      | 0.982<br>[0.951, 0.988]      | 0.986<br>[0.969, 0.995] | 0.955<br>[0.906, 0.976]         | 0.96<br>[0.919, 0.975]          |

**Supplementary Table S6.** Number of missing predictions (invalid or absent binary outputs) for the extraction of 13 clinical features from Persian palliative care transcripts across the evaluated small language models. Values are reported for Llama-3.1-8B-Instruct, Qwen2.5-7B-Instruct, Llama-3.2-3B-Instruct, Qwen2.5-1.5B-Instruct, Gemma-3-1B-IT, and Aya-expense-8B (English-translated and direct Persian variants); missing cases were imputed as negative (False) in performance analyses.

| <i>features</i>                         | <i>Llama-3.1-8B-Instruct</i> | <i>Qwen2.5-7b-Instruct</i> | <i>Llama-3.2-3B-Instruct</i> | <i>Qwen2.5-1.5B-Instruct</i> | <i>Gemma-3-1b-it</i> | <i>Aya-expense-8b (English)</i> | <i>Aya-expense-8b (Persian)</i> |
|-----------------------------------------|------------------------------|----------------------------|------------------------------|------------------------------|----------------------|---------------------------------|---------------------------------|
| <i>Doctor's visit request</i>           | 1                            | 0                          | 1                            | 0                            | 208                  | 27                              | 38                              |
| <i>Psychological complaints</i>         | 1                            | 0                          | 1                            | 6                            | 209                  | 21                              | 38                              |
| <i>Sleep disorders</i>                  | 1                            | 0                          | 1                            | 0                            | 205                  | 26                              | 38                              |
| <i>Loss of appetite</i>                 | 1                            | 0                          | 1                            | 0                            | 205                  | 28                              | 38                              |
| <i>Seizures</i>                         | 1                            | 0                          | 1                            | 0                            | 205                  | 26                              | 39                              |
| <i>Weakness and fatigue</i>             | 1                            | 0                          | 1                            | 0                            | 205                  | 27                              | 38                              |
| <i>Decreased level of consciousness</i> | 1                            | 0                          | 1                            | 0                            | 206                  | 27                              | 38                              |
| <i>Fever</i>                            | 1                            | 0                          | 1                            | 0                            | 205                  | 29                              | 40                              |
| <i>Respiratory complaints</i>           | 1                            | 0                          | 1                            | 0                            | 209                  | 28                              | 38                              |
| <i>Insurance/treatment cost issues</i>  | 1                            | 0                          | 1                            | 0                            | 205                  | 31                              | 40                              |
| <i>Urinary tract issues</i>             | 1                            | 0                          | 1                            | 0                            | 205                  | 31                              | 39                              |
| <i>Pain</i>                             | 1                            | 0                          | 1                            | 0                            | 205                  | 37                              | 40                              |
| <i>Gastrointestinal issues</i>          | 1                            | 0                          | 1                            | 0                            | 206                  | 30                              | 39                              |

**Supplementary Table 7.** Matthews Correlation Coefficients (MCC) for the binary extraction of 13 clinical features from Persian palliative care transcripts across the evaluated small language models. Values are reported for Llama-3.1-8B-Instruct, Qwen2.5-7B-Instruct, Llama-3.2-3B-Instruct, Qwen2.5-1.5B-Instruct, Gemma-3-1B-IT, and Aya-expans-8B (English-translated and direct Persian variants).

| <i>features</i>                             | <i>Llama<br/>-3.1-<br/>8B-<br/>Instru<br/>ct</i> | <i>Qwen2.<br/>5-7b-<br/>Instruct</i> | <i>Llama<br/>-3.2-<br/>3B-<br/>Instru<br/>ct</i> | <i>Qwen2.<br/>5-1.5B-<br/>Instruct</i> | <i>Gemm<br/>a-3-1b-<br/>it</i> | <i>Aya-<br/>expans<br/>e-8b<br/>English</i> | <i>Aya-<br/>expans<br/>e-8b<br/>Persian</i> |
|---------------------------------------------|--------------------------------------------------|--------------------------------------|--------------------------------------------------|----------------------------------------|--------------------------------|---------------------------------------------|---------------------------------------------|
| <i>Doctor's visit<br/>request</i>           | <b>0.664</b>                                     | 0.445                                | 0.488                                            | 0.501                                  | 0.361                          | 0.229                                       | 0.197                                       |
| <i>Psychological<br/>complaints</i>         | 0.672                                            | 0.670                                | 0.656                                            | 0.604                                  | 0.565                          | <b>0.673</b>                                | 0.719                                       |
| <i>Sleep disorders</i>                      | 0.632                                            | <b>0.683</b>                         | 0.572                                            | 0.589                                  | 0.502                          | 0.531                                       | 0.584                                       |
| <i>Loss of appetite</i>                     | 0.818                                            | <b>0.832</b>                         | 0.791                                            | 0.751                                  | 0.496                          | 0.744                                       | 0.760                                       |
| <i>Seizures</i>                             | 0.751                                            | <b>0.817</b>                         | 0.761                                            | 0.654                                  | 0.581                          | 0.751                                       | 0.618                                       |
| <i>Weakness and<br/>fatigue</i>             | 0.794                                            | 0.820                                | 0.733                                            | <b>0.842</b>                           | 0.730                          | 0.582                                       | 0.573                                       |
| <i>Decreased level<br/>of consciousness</i> | 0.620                                            | <b>0.819</b>                         | 0.587                                            | 0.645                                  | 0.518                          | 0.704                                       | 0.641                                       |
| <i>Fever</i>                                | 0.821                                            | <b>0.850</b>                         | 0.821                                            | 0.847                                  | 0.734                          | 0.794                                       | 0.842                                       |
| <i>Respiratory<br/>complaints</i>           | <b>0.842</b>                                     | 0.791                                | 0.825                                            | 0.772                                  | 0.428                          | 0.818                                       | 0.837                                       |
| <i>Insurance/treatm<br/>ent cost issues</i> | 0.670                                            | <b>0.797</b>                         | 0.737                                            | 0.582                                  | 0.398                          | 0.757                                       | 0.442                                       |
| <i>Urinary tract<br/>issues</i>             | 0.742                                            | 0.637                                | 0.734                                            | 0.574                                  | 0.312                          | <b>0.776</b>                                | 0.686                                       |
| <i>Pain</i>                                 | <b>0.864</b>                                     | 0.808                                | 0.787                                            | 0.753                                  | 0.660                          | 0.724                                       | 0.757                                       |
| <i>Gastrointestinal<br/>issues</i>          | <b>0.749</b>                                     | 0.659                                | 0.696                                            | 0.661                                  | 0.394                          | 0.634                                       | 0.699                                       |
| <i>Median [IQR1<br/>,IQR3]</i>              | 0.749<br>[0.67,<br>0.818]                        | 0.797<br>[0.67,<br>0.819]            | 0.734<br>[0.656,<br>0.787]                       | 0.654<br>[0.589,<br>0.753]             | 0.502<br>[0.398,<br>0.581]     | 0.724<br>[0.634,<br>0.757]                  | 0.686<br>[0.584,<br>0.757]                  |
